# Supplementary material for: Dual approach to soft-core anyonic Lieb-Liniger fluids
Source: arXiv:2407.06108 source file (2024-07-08)
Supplement: Supplementary file 1 [file Appendix.tex]

\clearpage
%\newpage

\onecolumngrid

\appendix

\centerline{\large \bf Supplementary information for ``Dual approach to soft-core anyonic Lieb-Liniger fluids''}

\centerline{}

\centerline{Gerard Valentí-Rojas and Patrik Öhberg}

%\tableofcontents

\section{Dual Mapping}

\section{Dimensional Reduction Arguments}

\section{Bogoliubov Analysis}

\section{Quantum Hydrodynamics}

\section{Numerical Simulations}
%%%%%%%%%%%%%%%%%%%%%%%%%%%%%%%%%%%%%%%%%%%%%%%%%%%
\begin{figure*}[th]
%\centering
    \includegraphics[width=0.48\textwidth]{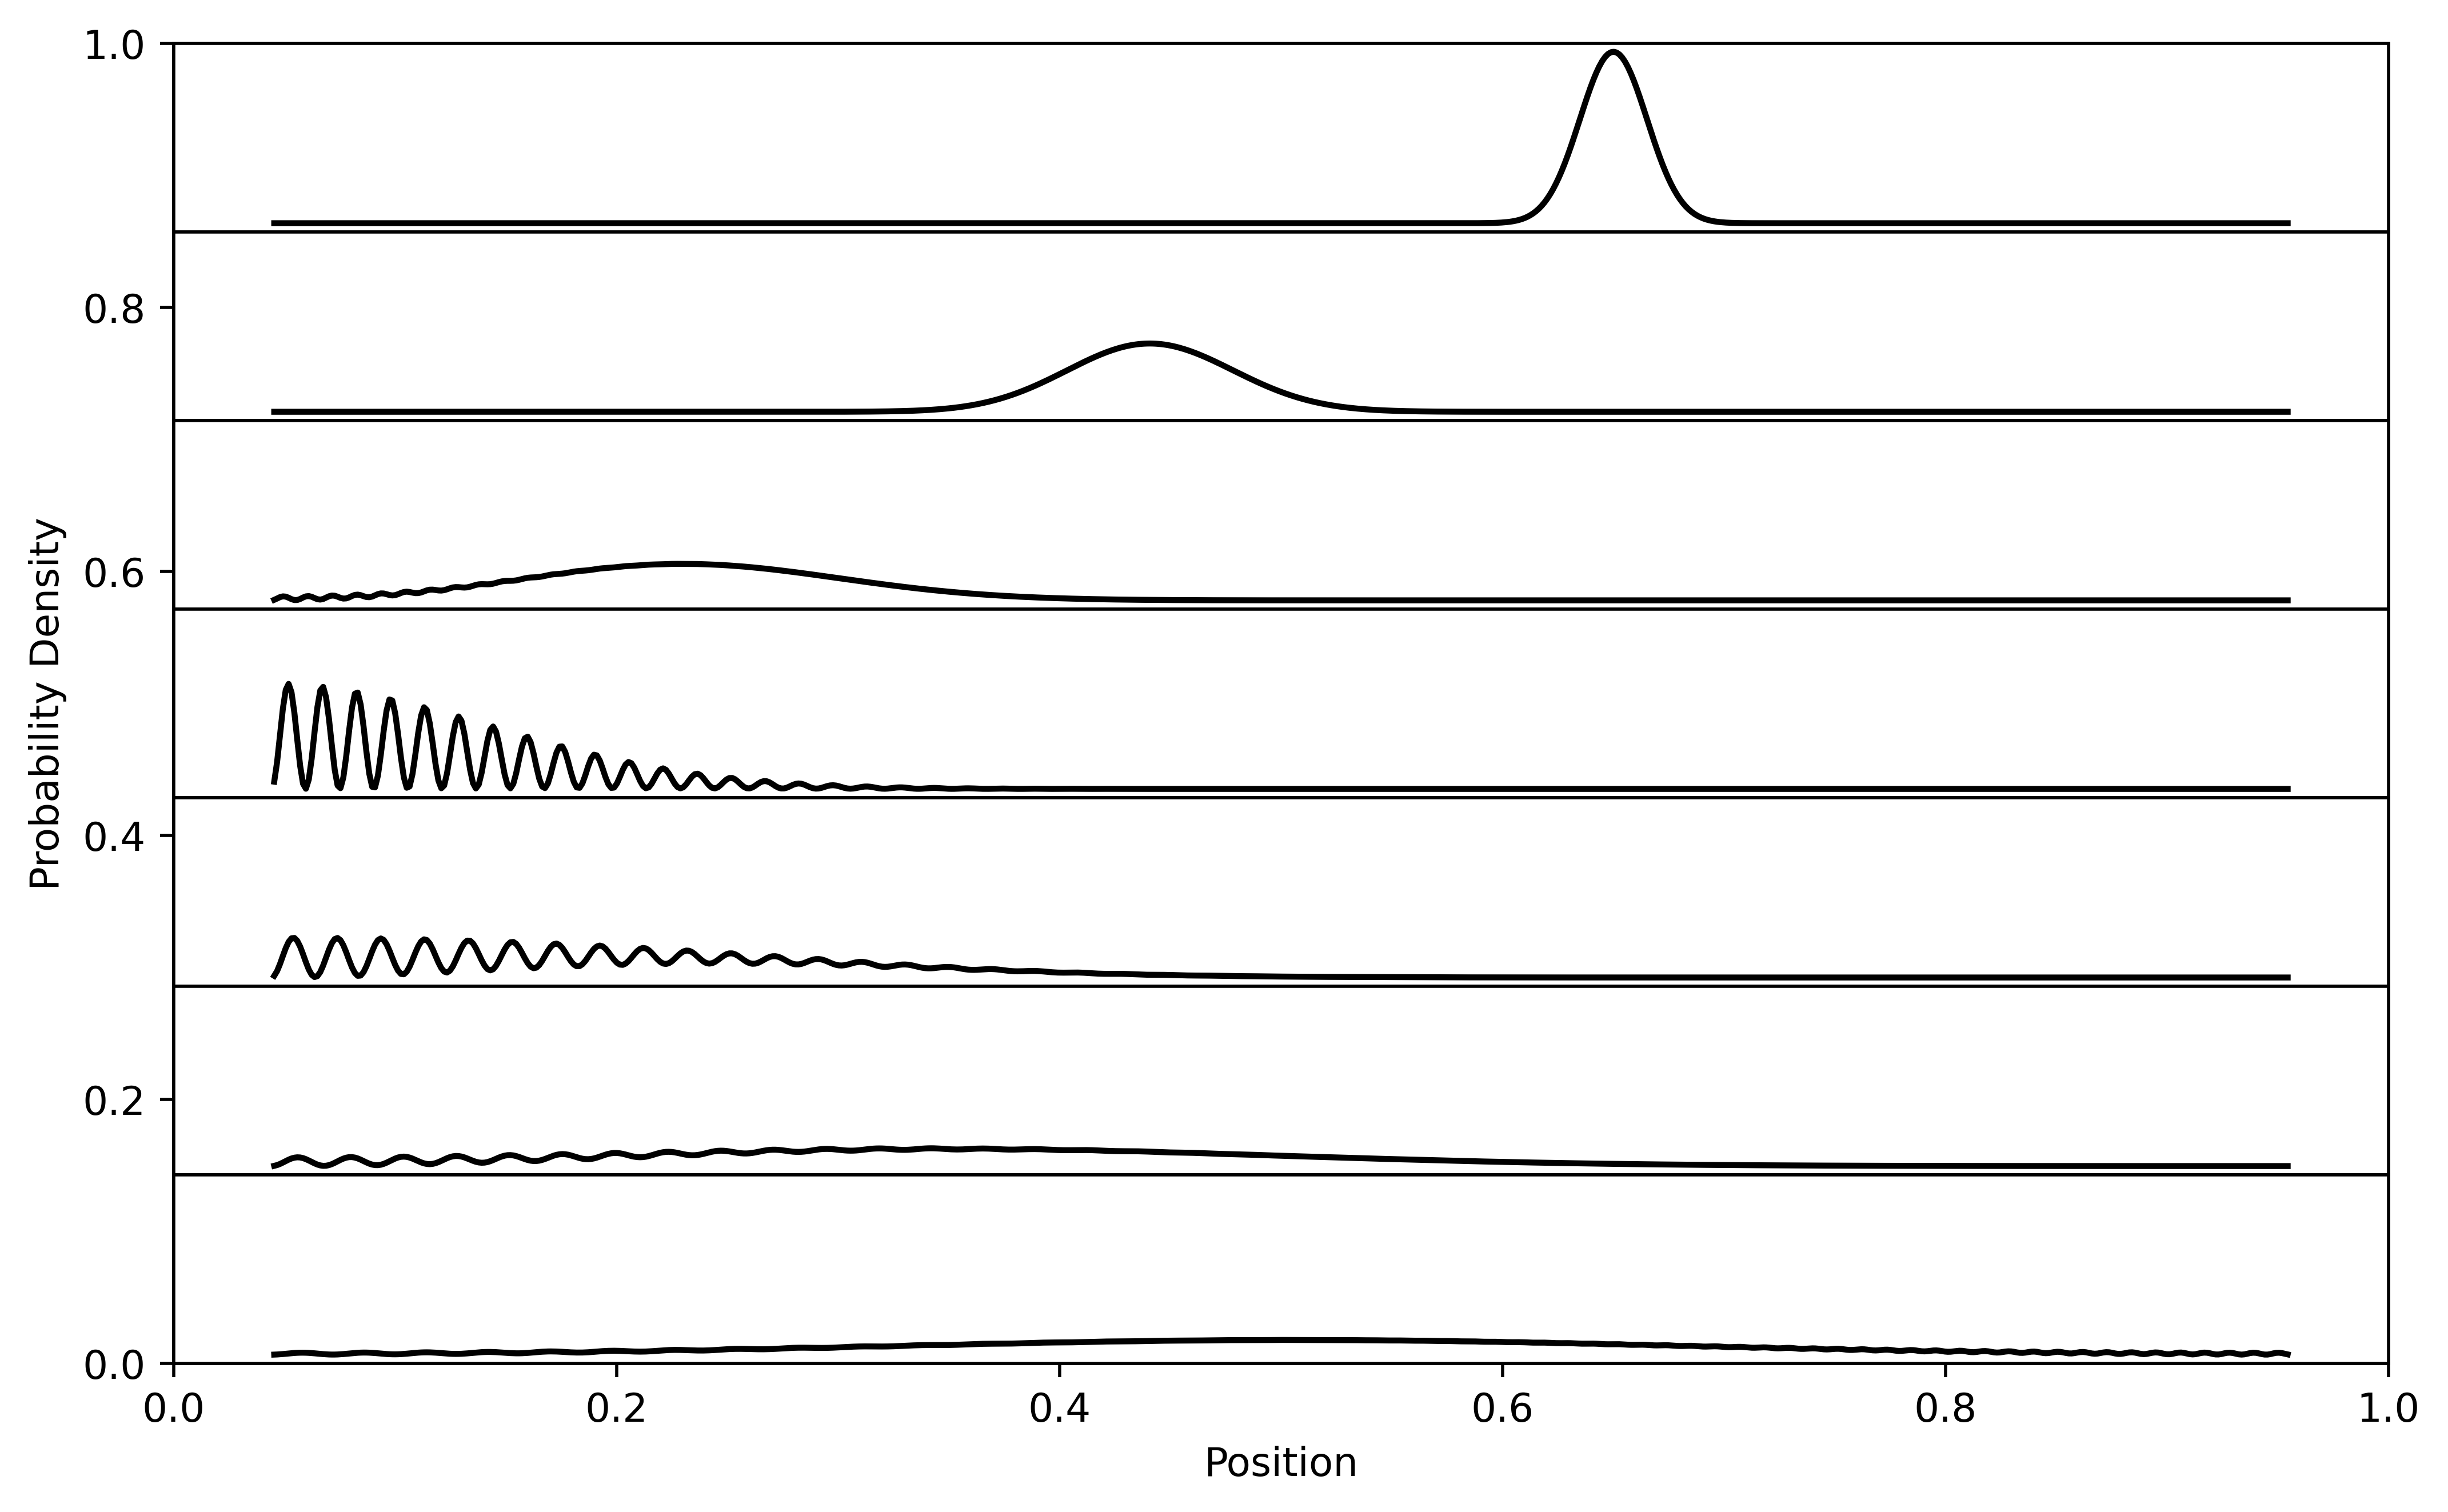}
    \hspace{0.3cm}
    \includegraphics[width=0.48\textwidth]{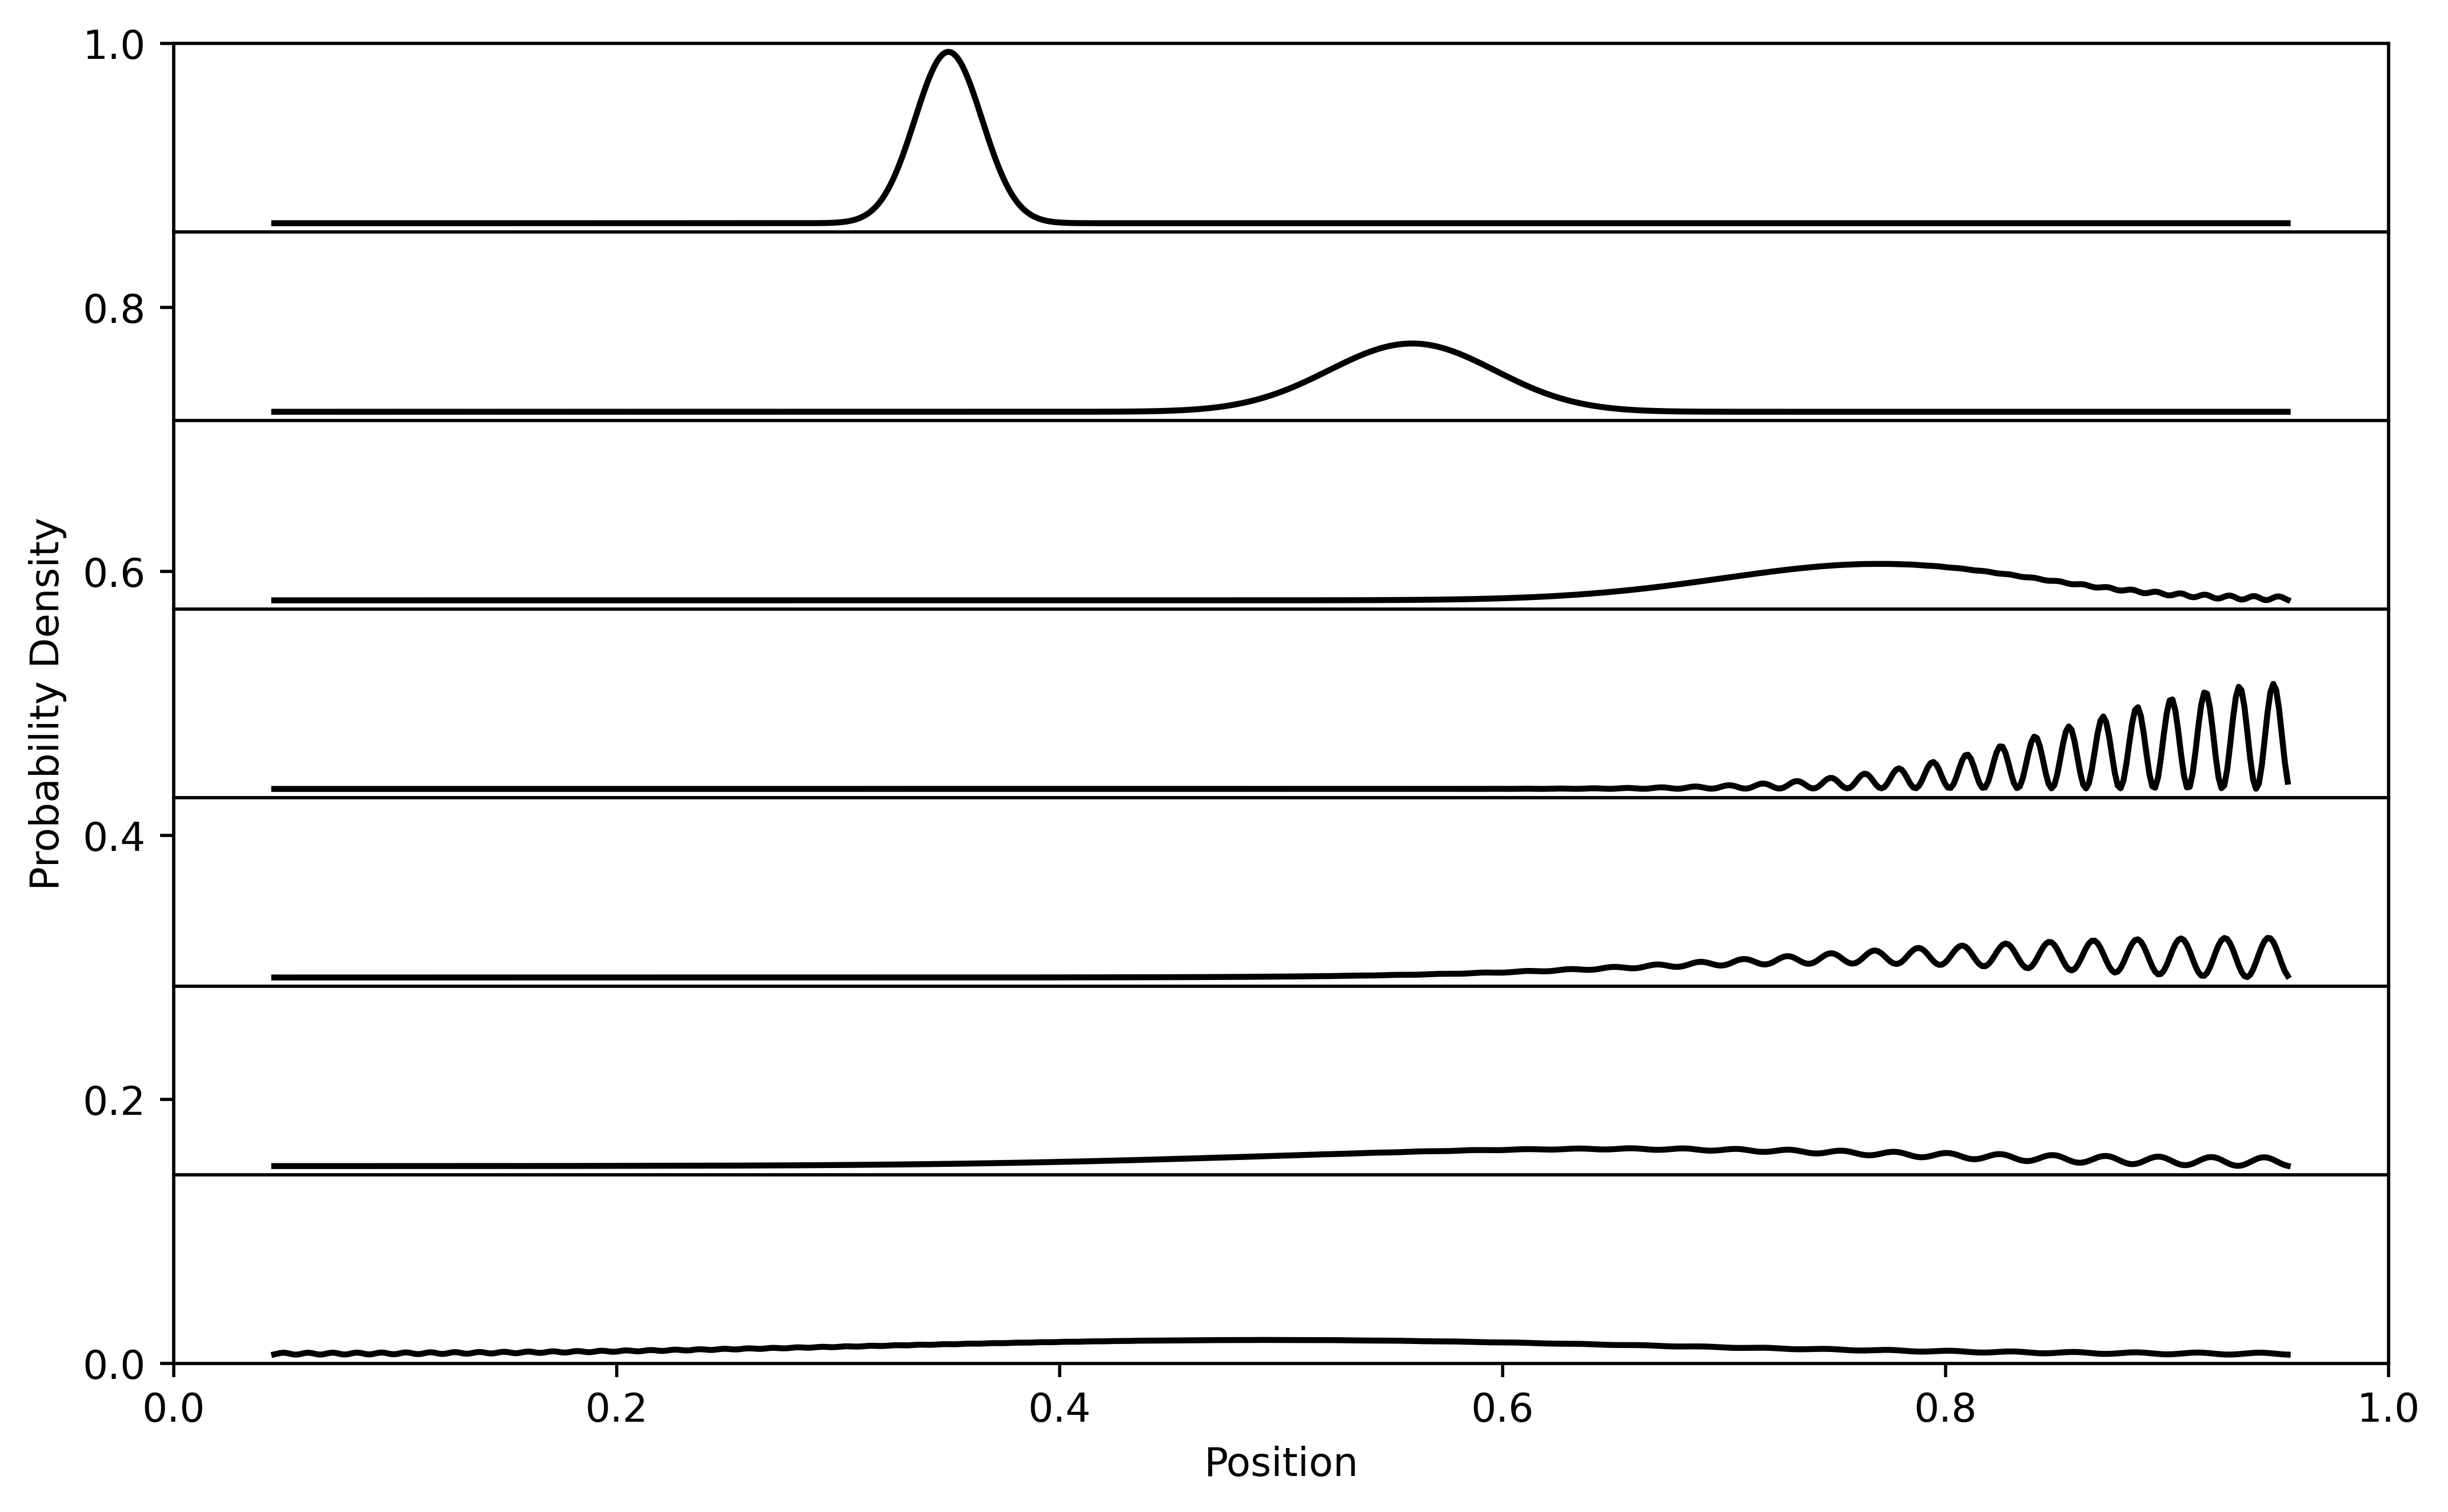}
    \caption{(\textit{Left}) Conventional reflection dynamics for Gross-Pitaevskii wavepacket for a $k<0$ kick. The wavepacket presents self-interference upon backscattering with a wall. After bouncing off, the conventional density profile is recovered and interference effects disappear. (\textit{Right}) Similar dynamics for a $k>0$ kick.}
   \label{fig:same}
\end{figure*}
